# Supplementary material for: Cops and Robbers on Intersection Graphs
Source: arXiv:1607.08058 source file (2016-07-27)
Supplement: Supplementary file 1 [file appendix.tex]

\appendix
\section*{Appendix}

In this section we present the more technical proofs and remarks.

\begin{proof}[Lemma~\ref{lem:path-neighbourhood}]
    We assume a cop's strategy $\mathcal{S}$ as given by Lemma~\ref{lem:shortest-path}
    and describe a new strategy for five cops. In the rest of the proof, we assume any
    cop happening to be adjacent to the robber will capture him immediately.

    The cop $C_0$ moves according to $\mathcal{S}$. When $C_0$ moves to $p_i$,
    the cops $C_j$  for $j \in \{-2, -1, 1, 2\}$ move to $p_{i+j}$. This is always possible
    since $\mathcal{S}$ moves $C_0$ only by distance one and on the path $P$.
    In case a cop would have to move beyond $P$'s endpoints, he just stays on the endpoint.
    This way the cops always occupy five consecutive vertices of the path
    (or share an endpoint of the path).

    Now assume that the robber moves to a vertex $r$. If $r$ is adjacent to
    a vertex $q$, which is in turn adjacent to $p_i$, strategy $\mathcal{S}$
    moves $C_0$ to one of $p_{i-2}\dots p_{i+2}$, since otherwise the robber could step on
    $P$ in two moves without being immediately captured by $C_0$, but that contradicts the
    properties of $\mathcal{S}$. Therefore, after the cops' move, there is at least one
    cop on $p_i$, and so if the robber moves to $q$, he is captured immediately.
    Note that this argument holds for every such $q$ and $p_i$.

    The initial setup procedure is almost identical to the one in
    Lemma~\ref{lem:shortest-path} -- the cops first all meet on $p_0$, say, and 
    then move towards their vertices prescribed by the strategy above.
    Even though their prescribed vertices may move while they are on their way,
    the prescribed vertices move only on $P$ and only with speed at mos one,
    so every cop will assume his position and start guarding in at most
    $|P|$ turns after meeting at $p_0$. \qed
\end{proof}

\smallskip
To guard a path $P$ with cops only moving on $P$ (unless immediately capturing the robber),
we can show that five cops are necessary as shown in Fig.~\ref{fig:five-neccessary}.
With the robber on $r$, there needs to be a cop on each of the vertices $p_{i-2}\dots p_{i+2}$.

\begin{figure}[hbt]
    \centering
    \includegraphics{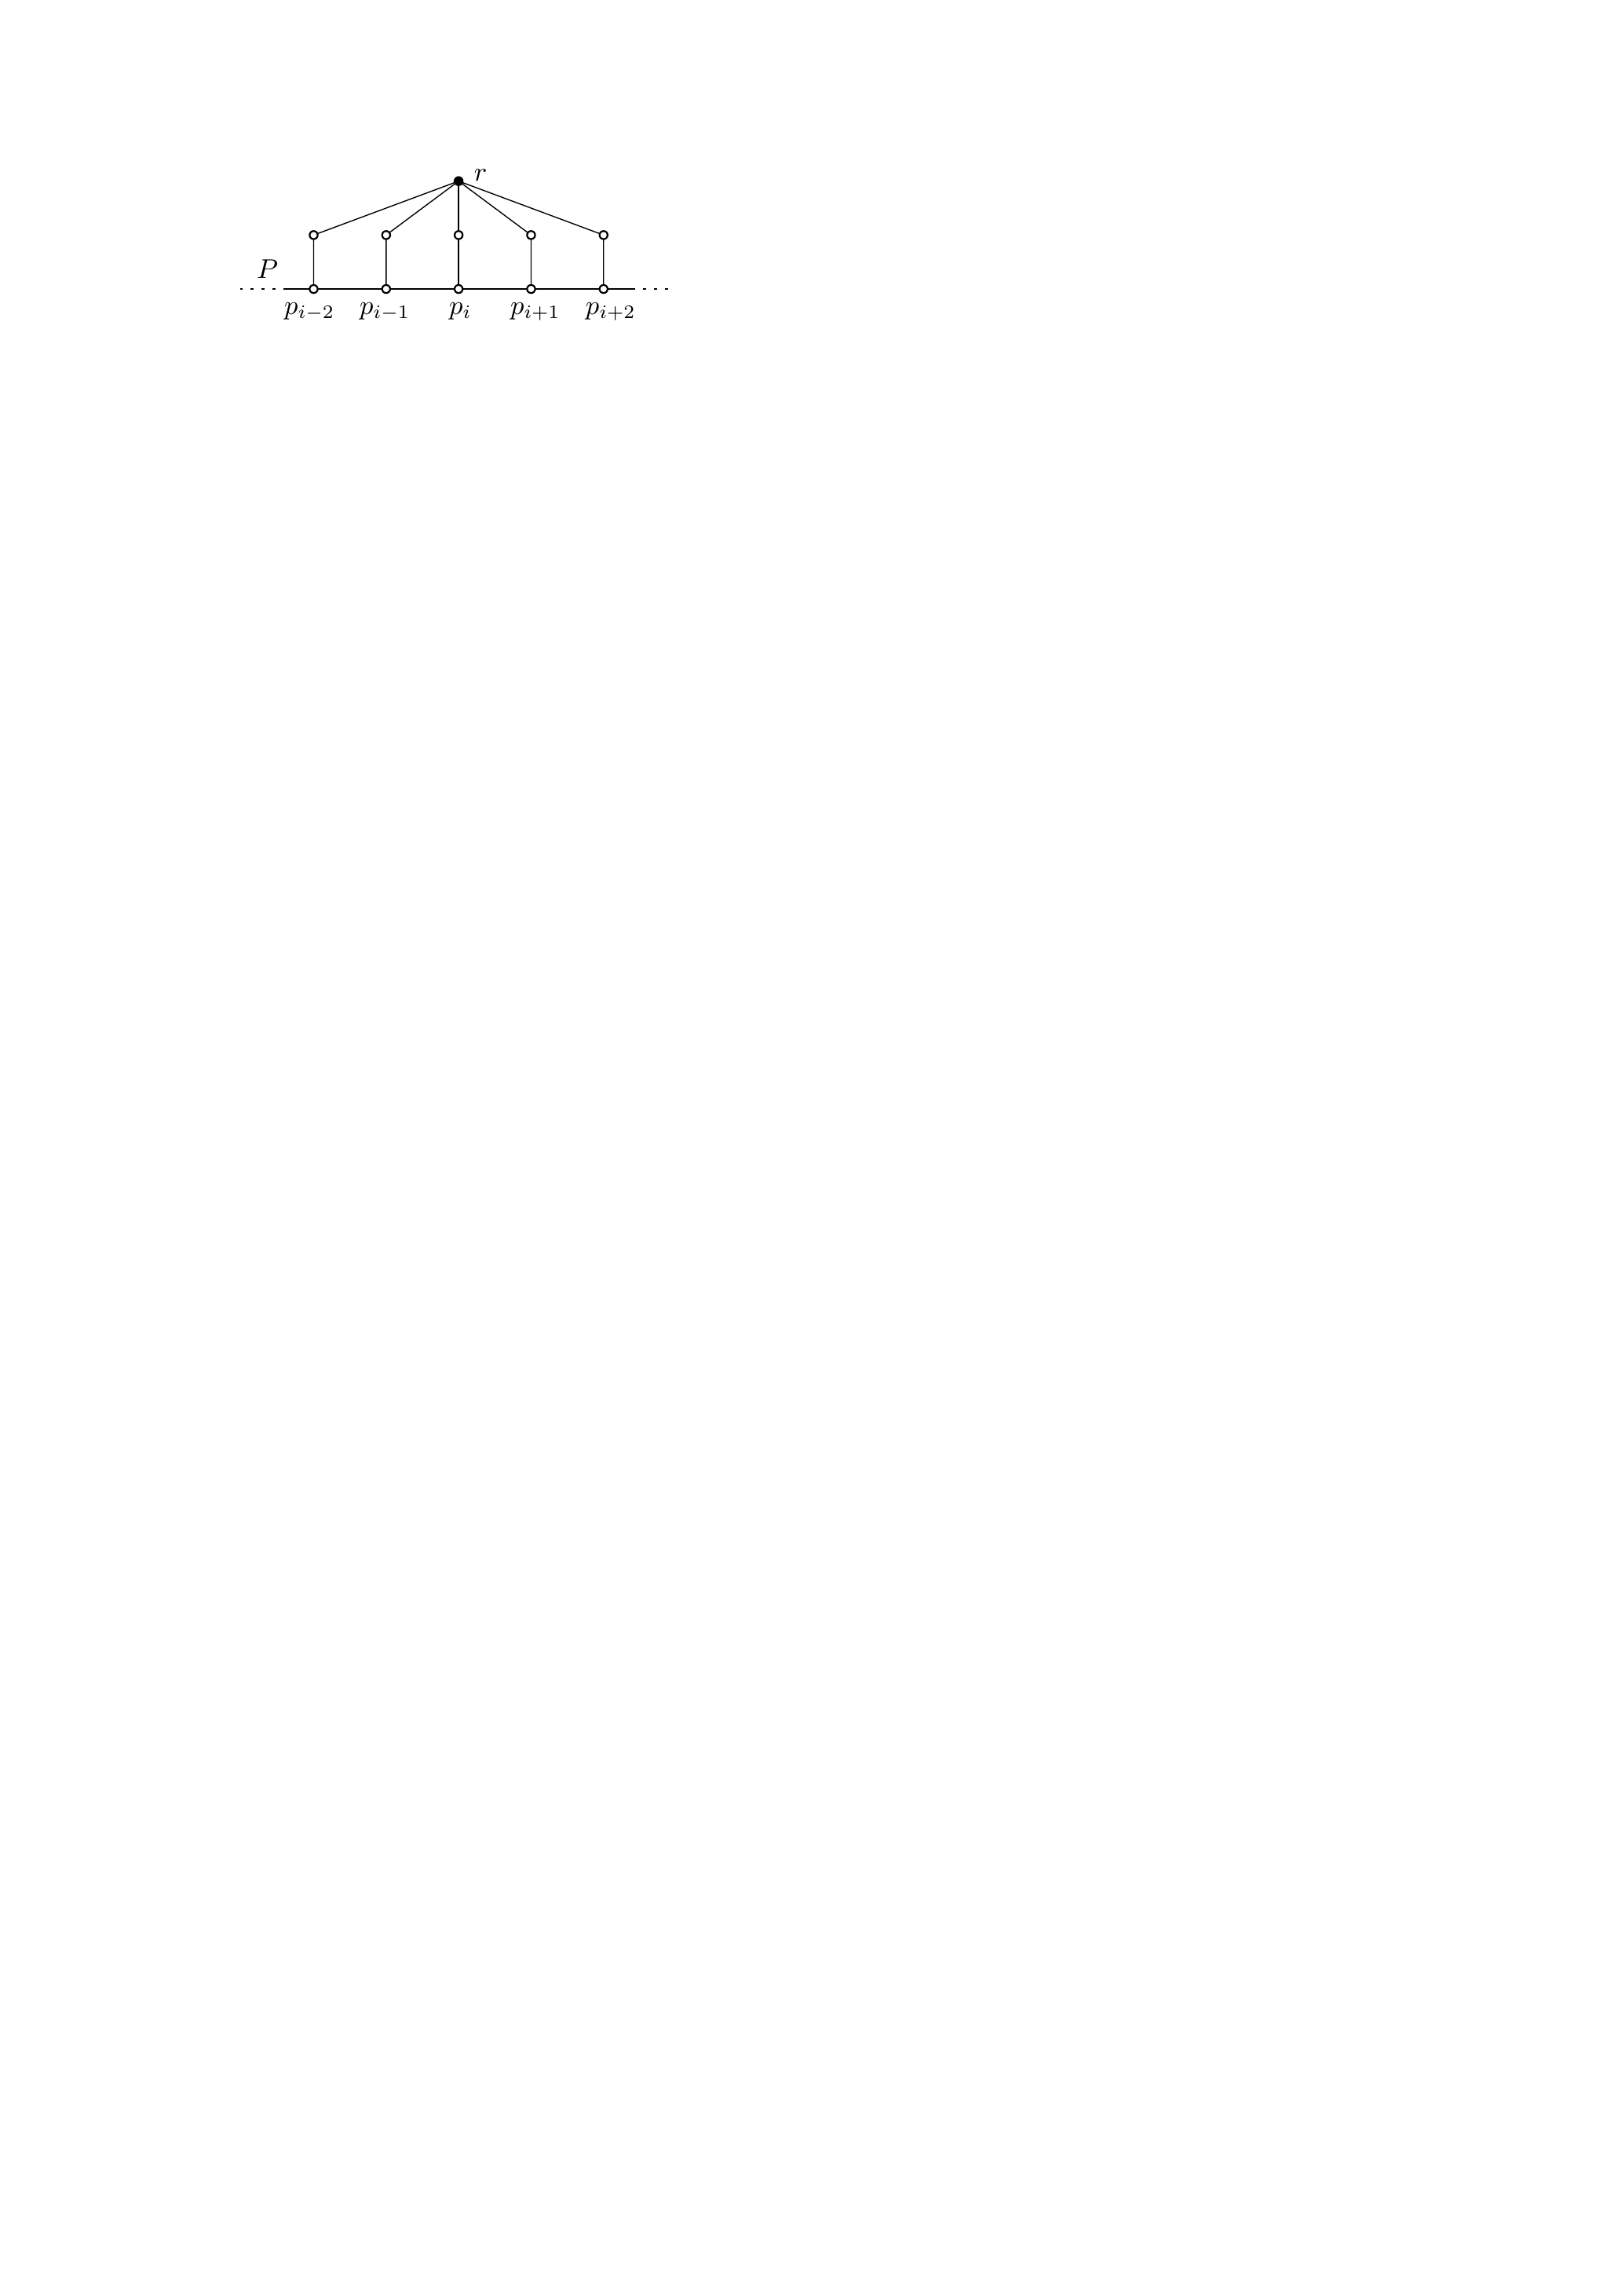}
    \caption{A situation illustrating the necessity of five cops to guard $P$.}
    \label{fig:five-neccessary}
\end{figure}

\begin{proof}[Claim in Theorem~\ref{thm:string_strategy}]
    {\it Base cases.} If $|\A(\varphi(V))|=1$, $\varphi(V_{S_{abc}})$ does not contain a (topological) cycle and therefore
    $V_{S_{abc}}$ form a forest. It is not difficult to see that one cop can capture the robber in a forest.
    In case $|V_{S_{abc}}|\leq 15$, the cops can occupy every vertex of $V_{S_{abc}}$, capturing the robber.
    Below we assume $|V_{S_{abc}}|>15$ and $|\A(\varphi(V))|>1$.

    \smallskip
    {\it Case 1.} If there is a shortest curve $\pi_{db}$ between a point $\pi_d\in\pi_{ac}$ and the point $\pi_b$ such that it divides
    $S_{abc}$ into at least two non-empty regions, choose $\pi_{db}$ such that the only intersection with $\pi_{ac}$
    is $\pi_d$ (this can be done by removing all $\pi_{db}$ before the last intersection with $\pi_{ac}$) and
    that has at most one meeting with each of $\pi_{ab}$ and $\pi_{bc}$ (using Lemma~\ref{lem:meet-once}).
    Now use five cops to guard $\pi_{db}$ and see in which region of $\A(\pi_{abc}\cup\pi_{db})$ the robber is.
  
    See Fig.~\ref{fig:claim-curve-db} and notice that each of the possible regions is
    bounded by two or three sub-curves of $\pi_{ab}$, $\pi_{bc}$, $\pi_{ca}$ and $\pi_{db}$.
    Let $\pi_{ef}$, $\pi_{fg}$ and $\pi_{ge}$ be such sub-curves forming a simple triangle
    $\pi_{efg}=\pi_{ef}\cup\pi_{fg}\cup\pi_{ge}$.
    In case there were only two sub-curves, arbitrarily divide one of them into non-zero length parts to get
    three sub-curves. Now transition to guarding $\pi_{ef}$, $\pi_{fg}$ and $\pi_{ge}$ instead of the previously
    guarded curves. Such transition is possible without additional cops since the cops guarding a curve also
    simultaneously guard all of its sub-curves, so we only need to limit the cops to the smaller range.
    
    Let $S_{efg}$ be the region inside $\pi_{efg}$ and let $G'=G|_{\C(S_{efg})}$.
    Since the curves $\pi_{ef}$, $\pi_{fg}$ and $\pi_{ge}$ stay shortest in $G'$ and $S_{efg}\subsetneq S_{abc}$,
    we may apply the inductive argument and get a strategy capturing the robber in $G'$ with $\pi_{ef}$, $\pi_{fg}$ and $\pi_{ge}$
    guarded and using Lemma~\ref{lem:restrict-strategy} we get a strategy for $G$ with $\pi_{ef}$, $\pi_{fg}$ and $\pi_{ge}$ 
    guarded.
    
    \begin{figure}[ht]
	\centering
	\includegraphics{fig-claim-curve-db.pdf}
	\caption{
	The first case in the proof the claim in proof of
	Theorem~\ref{thm:string_strategy}.
	Note that $\pi_{bd}$ may not meet either of $\pi_{ab}$ or $\pi_{bc}$ or
	$\pi_{bd}$ could first meet $\pi_{ab}$ and then $\pi_{bc}$.}
	\label{fig:claim-curve-db}
    \end{figure}

    \smallskip
    {\it Case 2.}
    Let $V'\subseteq V$ be the vertices not used in any of the underlying paths of
    $\pi_{abc}$. Now choose $d\in V'$ and $\pi_d\in\varphi(d)$. Also choose three shortest curves $\pi_{ad}$, $\pi_{bd}$ and
    $\pi_{cd}$ from $\pi_d$ to $\pi_{a}$, $\pi_{b}$ and $\pi_{c}$ respectively. Using Lemma~\ref{lem:meet-once}, we may
    assume that each of $\pi_{ad}$, $\pi_{bd}$, $\pi_{cd}$ meets each of $\pi_{ab}$, $\pi_{bc}$, $\pi_{ca}$ at most once.
    Observe that $\pi_{ad}$, $\pi_{bd}$, $\pi_{cd}$ may not cross $\pi_{abc}$, so each of their intersections with
    $\pi_{abc}$ is either their endpoint or a meeting.
    Since we solved Case 1 above, we may assume that if $\pi_{da}$ meets $\pi_{bc}$, it never leaves $\pi_{abc}$ before
    ending in $\pi_{a}$, and similarly for $\pi_{db}$ and $\pi_{dc}$.

    Now let 15 cops guard $\pi_{ad}$, $\pi_{bd}$, $\pi_{cd}$. Below we reference $\pi_{ab}$, $\pi_{bc}$, $\pi_{ca}$,
    $\pi_{ad}$, $\pi_{bd}$ and $\pi_{cd}$ as the \emph{guarded curves}.
    Let $r$ be the vertex with the robber after the manoeuvre.
    If $\varphi(r)\cap(\pi_{abc}\cup\pi_{ad}\cup\pi_{bd}\cup\pi_{cd})\neq\emptyset$ the robber will be captured in the
    next turn, so we assume $\varphi(r)\subseteq R\in\A(\pi_{abc}\cup\pi_{ad}\cup\pi_{bd}\cup\pi_{cd})$.
    The following lemma is a little technical, the proof can be found below.

    \begin{lemma}\label{lem:three-sub-curves}
    In the situation as above, there are three sub-curves $\pi_{ef}$, $\pi_{fg}$ and $\pi_{ge}$ of the guarded curves,
    with $\pi_{efg}=\pi_{ef}\cup\pi_{fg}\cup\pi_{ge}$ a simple closed curve containing entire $R$ inside.
    Additionally, we have that at most one of $\pi_{ef}$, $\pi_{fg}$ and $\pi_{ge}$ is a sub-curve of
    $\pi_{abc}-(\pi_{ad}\cup\pi_{bd}\cup\pi_{cd})$.
    \end{lemma}

    \smallskip
    Now if the interior $S_{efg}$ of $\pi_{efg}=\pi_{ef}\cup\pi_{fg}\cup\pi_{ge}$ has strictly smaller area
    (or equivalently, fewer regions of $\A(\varphi(V))$) than $S_{abc}$,
    we may use the same argument as in Case 1 above -- move to guard only
    $\pi_{ef}$, $\pi_{fg}$ and $\pi_{ge}$, and then use the inductive argument on $G$ restricted to $\C(S_{efg})$ to get
    a winning strategy.

    \smallskip
    Whenever we have a component $C$ of $G|_{V'}$ with $|N(C)|\geq 2$, me may choose
    $\pi_d\in\varphi(C)$ and $\pi_{ad}$, $\pi_{bd}$ and $\pi_{cd}$ such that two of these curves leave
    $\varphi(C)$ via different vertices of $N(C)$. To find them take $n_1,n_2\in N(C)$ on different
    underlying paths of $\pi_{abc}$ if possible, say $\pi_{ab}$ and $\pi_{bc}$; in this case choose
    $n_1$ and $n_2$ closest to $\pi_a$ and $\pi_c$ (on the underlying paths) and find a shortes
    $n_1-n_2$ path in $C$. On this path, there is either a vertex or an edge with the same distance to
    $\pi_a$ and $\pi_c$, giving us the desired $\pi_{ad}$, $\pi_{cd}$. If all $N(C)$ lie on one of the
    underlying shortest paths, say $\pi_{ab}$, choose $n_1$ and $n_2$ closest to its endpoinds and get
    $\pi_{ad}$ and $\pi_{bd}$ similarly.
    However we then choose $\pi_{ef}$, $\pi_{fg}$ and $\pi_{ge}$, we always have the area of $S_{efg}$
    (or the number of contained regions of $\A(\varphi(V))$) strictly smaller than $S_{abc}$
    and we may apply the inductive argument.

    The only remaining case is when all the components of $V'$ have only one external neighbor.
    In this case let $C$ be the component of $G|_{V'}$ containing the robber and let $v\in N(C)$.
    Observe that $v$ is a cutvertex in $G$. Let the 15 cops stop guarding $\pi_{ad}$, $\pi_{bd}$ and $\pi_{cd}$
    and place one cop on $v$. Then, as long as there is $v'\in N(v)$ closer to the robber with $v'$ also a cutvertex,
    move the cop to $v'$. In this way the cop chases the robber in $C$ until he captures him or arrives on vertex $v''$
    with at least two neighbors in $C''$ which is the component of $G-\{v''\}$ cotaining the robber.
    Let $D$ be a shortest cycle in $C''$ containing $v''$ (e.g. using a shortest path in $C''$ connecting two neighbors of $v''$).
    Choose shortest curves $\pi_{ef}$, $\pi_{fg}$ and $\pi_{ge}$ in $\varphi(D)$ with $\pi_e\in\varphi(v)$ and forming a
    simple closed curve $\pi_{efg}$. We may now stop guarding $\pi_{abc}$ and guard $\pi_{ef}$, $\pi_{fg}$ and $\pi_{ge}$.
    Note that we may now remove the extra cop from $v''$. In case the robber is inside $\pi_{efg}$, use the inductive
    argument on $G|_{\C(S_{efg})}$, in case he is outside, apply circular inversion on $\varphi$ to get
    $\varphi'$ where the robber is inside $\pi'_{efg}$ and apply the same inductive argument on $G|_{\C(S'_{efg})}$ with $\varphi'$.
    \qed
%   \todo{Figure?}
\end{proof}

\begin{proof}[Lemma~\ref{lem:three-sub-curves}]
    \begin{figure}[ht]
	\centering
	\includegraphics{fig-claim-R-boundary.pdf}
	\hskip 7mm
	\includegraphics{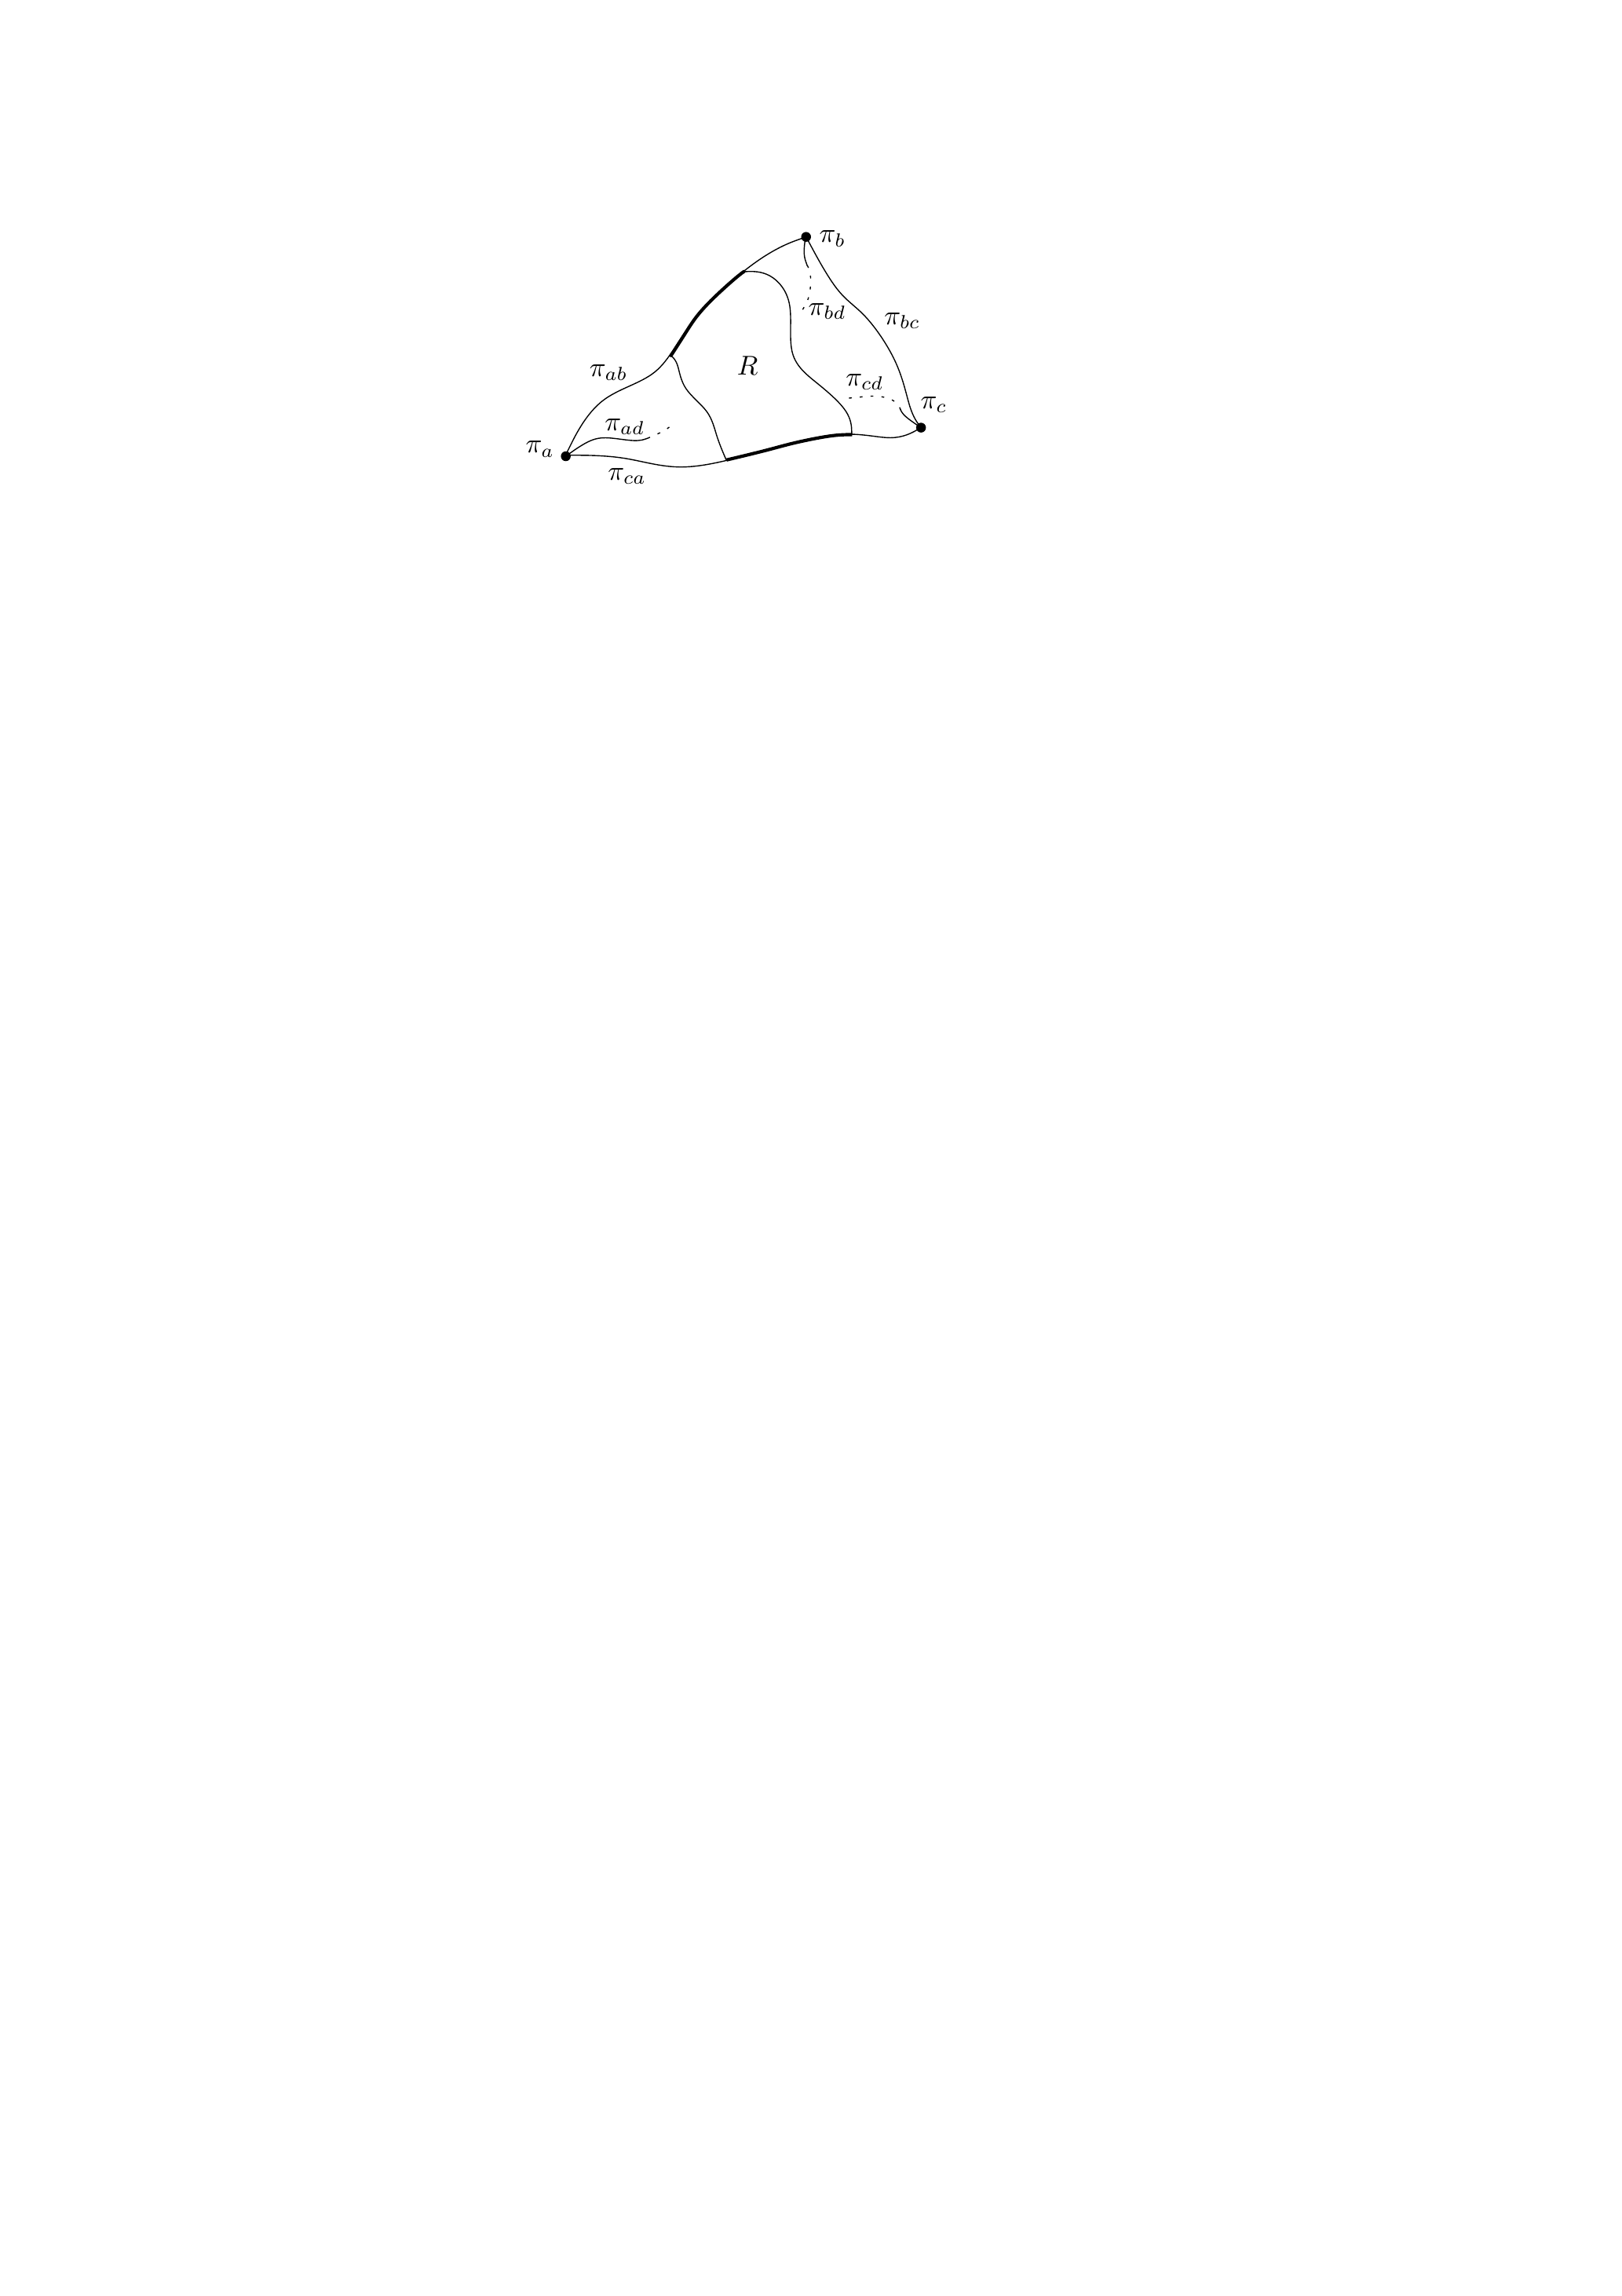}
	\caption{{\it Left:} An illustration of the boundary of the region $R$. $\pi^0$ consists of the thick
	curves. {\it Right:} $\pi_{*d}$ avoid both $R$ and the thick parts of $\pi_{ab}$ and $\pi_{ca}$,
	leading to contradiction with any position of $\pi_d$.}
	\label{fig:claim-R-boundary}
	\label{fig:curve-R-separates}
    \end{figure}

    \smallskip
    Let $\pi^0=\C(R)-R$ be the boundary of $R$. $\pi^0$ consists only of sub-curves of the guarded curves.
    Let $B^0=\{b^0_1\dots b^0_k\}$ be such sub-curves of the boundary of $R$ in a cyclic ordering and let
    $\Pi^0=\{\pi^0_1\dots\pi^0_k\}$ with $\pi^0_i$ the sub-curve that $b^0_i$ is part of.
    Whenever possible, prefer $\pi^0_i\not\in\{\pi_{ab},\pi_{bc},\pi_{ca}\}$ even if it requires larger $k$.
    See Fig.~\ref{fig:claim-R-boundary} for an illustration.

    Now we observe that $\Pi^0$ contains at most one of $\pi_{ab}$, $\pi_{bc}$ and $\pi_{ca}$.
    If it contained both, say, $\pi_{ab}$ and $\pi_{ca}$, $R$ together with $\C(R)\cap\pi_{abc}$ would separate
    $\pi_a$ from $\pi_b$ and $\pi_c$, a contradiction with their choice. See Fig.~\ref{fig:curve-R-separates}
    for an illustration of the situation.
    A very similar argument shows that $\Pi^0$ contains each of $\pi_{ab}$, $\pi_{bc}$ and $\pi_{ca}$ at most once.

    Now we choose a closed curve $\pi^1$ bounding $R$ such that it uses sub-curves only from three guarded curves.
    If $\Pi^0$ contains one instance of $\pi_{ab}$, $\pi_{bc}$ or $\pi_{ca}$, we may, without loss of generality,
    assume that it is $\pi_{ab}=\pi^0_1$ and let $b^0_1$ be this sub-curve. We note that $R$ is contained in
    one of the bounded regions of $\A(b^0_1\cup\pi_{ad}\cup\pi_{bd})$. For this note that
    $b^0_1$ touches $\pi_{ad}$ or $\pi_{bd}$ on both its ends since $\pi_{cd}$ does not touch
    $\pi_{ab}$ except perhaps in its endpoints.
    We choose $\pi^1$ to be any simple closed curve $b_1\cup\pi_{ad}\cup\pi_{bd}$ bounding $R$.
    In case $\Pi^0$ contains only $\pi_{ad}$, $\pi_{bd}$ and $\pi_{cd}$, we set $\pi^1=\pi^0$.
    In either case, we define $\Pi^1$ and $B^1$ similarly to $\Pi^0$ and $B^0$.

    \begin{figure}[ht]
	\centering
	\includegraphics{fig-claim-reduce-segments.pdf}
	\caption{An example how a closed curve $\pi^1$ (left; dashed) may be replaced by a closed curve $\pi^2$
	    (right; dashed) using only $s$ (the only outward-facing segment of $\pi^1-\pi_{ab}$)
	    and a part of $\pi_{ab}$.}
	\label{fig:claim-reduce-segments}
    \end{figure}

    Now we make sure that $|B|\leq3$. If, say $\pi_{ad}$, appears multiple times in $\Pi^1$, look at
    the segments of $\pi^1-\pi_{ad}$. Exactly one of them, denote it $s$, has the property that it is possible
    to start a new curve on this segment going outwards from $\pi^1$ and reach infinity without 
    crossing $\pi^1$ or $\pi_{ad}$. See Fig.~\ref{fig:claim-reduce-segments}.
    We may choose $\pi^2$ to consist of the sub-curves of $s$ and one sub-curve of $\pi_{ad}$ between the
    endpoints of $s$ (when taken as a curve). This gives us $\pi^2$ bounding $R$ using strictly less
    sub-curves of each of the guarded curves and $\pi_{ad}$ only once. We may repeat this for
    every guarded curve that appears in $\Pi^i$ more that once, getting $\pi^z$ together with $B^z$ and $\Pi^z$ and
    such that $2\leq|B^z|\leq 3$. In case $|B^z|=2$, we split any of the two curves of $B^z$, getting
    $\pi_{ef}$, $\pi_{fg}$ and $\pi_{ge}$ as advertised above. \qed
\end{proof}
